# Supplementary material for: Certifiably Robust Policy Learning against Adversarial Communication in Multi-agent Systems
Source: arXiv:2206.10158 source file (2022-07-02)
Supplement: Supplementary file 1 [file supp_macros.tex]

% Comments
\newcommand{\ys}[1]{{\color{blue}{YS:#1}}}
\newcommand{\rj}[1]{{\color{purple}{RJ:#1}}}
\newcommand{\draft}[1]{{\color{gray}{DRAFT:#1}}}
\newcommand{\fh}[1]{{\color{orange}{{#1}}}}
\newcommand{\fhc}[1]{{\color{orange}{\scriptsize{[FH:#1]}}}}
\newcommand{\change}[1]{{\color{red}{#1}}}
\newcommand{\SF}[1]{{\color{red}{SF:#1}}}

%%% functions
\newcommand{\natobj}{J_{\mathrm{nat}}}
\newcommand{\advobj}{J_{\mathrm{att}}}
\newcommand{\funabl}{\mathsf{Ablate}}
\newcommand{\funmed}{\mathsf{Median}}
\newcommand{\commfunc}{\xi}

%%% spaces
\newcommand{\agents}{\mathcal{D}}
\newcommand{\his}{\tau}
\newcommand{\hisspace}{\Gamma}

%%% others
\newcommand{\step}{^{(t)}}
\newcommand{\krv}{\mathcal{T}}
\newcommand{\robaction}{\widetilde{a}}

\newcommand{\ablpolicy}{\hat{\pi}}
\newcommand{\smpolicy}{\widetilde{\pi}}

\newcommand{\safeaction}{\mathcal{A}_{\mathrm{benign}}}
\newcommand{\safeactiondist}{\mathcal{A}_{\mathrm{benign}}^{\mathrm{d}}}
\newcommand{\safeactioncont}{\mathsf{Range}(\safeaction)}


%%% messages
\newcommand{\mtoi}{\mathbf{m}_{: \to i}}
\newcommand{\msg}{\mathbf{m}}
\newcommand{\msgk}{[\mathbf{m}]_k}
\newcommand{\allmsgk}{\mathcal{H}_{k}(\msg)}
\newcommand{\allmsgkd}{\mathcal{H}_{k,D}(\msg)}
\newcommand{\msgki}{[\mtoi]_k}
\newcommand{\allmsgki}{\mathcal{H}_{k}(\mtoi)}
\newcommand{\ablmi}{\hat{\mathbf{m}}^k_{i}}
\newcommand{\goodmsg}{\mathbf{m}_{\mathrm{benign}}}
\newcommand{\advmsg}{\mathbf{m}_{\mathrm{adv}}}
\newcommand{\goodmsgk}{[\mathbf{m}_{\mathrm{benign}}]_k}
\newcommand{\advmsgk}{[\mathbf{m}_{\mathrm{adv}}]_k}
\newcommand{\goodallmsgk}{\mathcal{H}_{k}(\goodmsg)}
\newcommand{\advallmsgk}{\mathcal{H}_{k}(\advmsg)}




%%% names
\newcommand{\oursfull}{{Ablated Message Ensemble}\xspace}
\newcommand{\ours}{{AME}\xspace}
\newcommand{\ablname}{{message-ablation policy}\xspace}
\newcommand{\ablnames}{{message-ablation policies}\xspace}
\newcommand{\ensname}{{message-ensemble policy}\xspace}
\newcommand{\ablnamecap}{{Message-Ablation Policy}\xspace}
\newcommand{\ensnamecap}{{Message-Ensemble Policy}\xspace}
\newcommand{\safename}{{benign action}\xspace}
\newcommand{\ksample}{{k-sample}\xspace}
\newcommand{\ksamples}{{k-samples}\xspace}


\newcommand{\permute}{{Perm-Attack}\xspace}
\newcommand{\swap}{{Swap-Attack}\xspace}
\newcommand{\flip}{{Flip-Attack}\xspace}

\newcommand{\marketenv}{{InventoryManager}\xspace}
\newcommand{\mnistenv}{{MARL-MNIST}\xspace}

\newcommand{\argmin}{\operatornamewithlimits{argmin}}
\newcommand{\argmax}{\operatornamewithlimits{argmax}}

\definecolor{darkpastelgreen}{rgb}{0.01, 0.75, 0.24}

\newcommand{\myst}[1]{\textcolor{red}{\st{#1}}}
