# Supplementary material for: Certifiably Robust Policy Learning against Adversarial Communication in Multi-agent Systems
Source: arXiv:2206.10158 source file (2022-07-02)
Supplement: Supplementary file 2 [file supp_packages.tex]

% \usepackage{hyperref}
\usepackage{url}
% \usepackage{natbib}
\usepackage{graphicx}
% \usepackage{amsfonts}
% \usepackage{amsmath}
% \usepackage{amsthm}
\usepackage{bbm}
\usepackage{xcolor}
% \usepackage{algorithm}
\usepackage{scalerel}
% \usepackage[noend]{algpseudocode}
\setlength\parindent{0pt}

% \usepackage{natbib}
\usepackage[outdir=./]{epstopdf}
\usepackage{graphicx,float,pgfplots,wrapfig,sidecap,lipsum}

\usepackage{colortbl}
\usepackage{tablefootnote}
%\usepackage{subfig}
\usepackage[font=small,labelfont=bf]{caption}
\usepackage{subcaption}
\usepackage{subfloat}
% \usepackage{hyperref,psfrag} % not allowed by AAAI
\usepackage{tikz}
\usetikzlibrary{fit}
\usetikzlibrary{calc,shapes}
\usetikzlibrary{decorations.pathmorphing} % noisy shapes
\usetikzlibrary{fit}					% fitting shapes to coordinates
\usetikzlibrary{backgrounds}	% drawing the background after the foreground
\usetikzlibrary{pgfplots.groupplots}

\usepackage[utf8]{inputenc}
\usepackage{pgfplots}
\DeclareUnicodeCharacter{2212}{−}
\usepgfplotslibrary{groupplots,dateplot}
\usetikzlibrary{patterns,shapes.arrows}
\pgfplotsset{compat=newest}

\usepackage{xspace}
\usepackage{soul}
